# Supplementary material for: Multi-Scale Zero-Order Optimization of Smooth Functions in an RKHS
Source: arXiv:2005.04832 source file (2020-05-11)
Supplement: Supplementary file 1 [file appendix_Temp.tex]

\begin{lemma}
\label{lemma:smooth4}
Under the event $\mc{E}$, and for $n$ large enough, we have the following bounds:
\begin{itemize}
    \item For $K=\kse$ and $K=\kmat$ with $2\nu> (D+1)(D+4)$, we have the trivial bound $n_1 \leq n$. 
    \item For $K=\kmat$ with $2 \nu\leq (D+1)(D+4)$ we have $n_1 \leq n/2$.
\end{itemize}
\end{lemma}

\begin{proof} Define $j_0 = \lceil \log(\sqrt{n}/\igain)/\log(2) \rceil$. From \lemmaref{lemma:smooth2}, we know that the number of times a cell $E$ with radius $r_E = 2^{-j}$ for $j  \leq j_0$ is evaluated is upper bounded by $m_E = 2 \log(2/\delta_{T_n})/(8D2^{-2j\alpha})$. By plugging in the value of $\delta_{T_n}$ we have $m_E \leq C_8 2^{2j\alpha}$ where  $ C_8 = \frac{ \log(n^4 2^{4D} \pi^2/3 \delta)}{8D}$. Since the  number of cells with radius $2^{-j}$ can be trivially upper bounded by $2^{jD}$, we have the following:
\begin{align*}
    n_1 & \leq \sum_{j=0}^{j_0}C_8 2^{2j \alpha} 2^{jD} =C_8\lp  2^{j_0(D+2\alpha)} - 1 \rp \leq C_8 2^{j_0(D+2\alpha)} 
 \stackrel{(a)}{\leq}  C_8 \lp \frac{\sqrt{n}}{\igain}  \rp^{D+2\alpha}. 
\end{align*}

Now, suppose $\igain = n^{a}$ for some $a \in [0,1)$. Then we have $n_1 = \tOh{n^{(1/2-a)(D+2\alpha)}}$. Consider the following cases:
\begin{itemize}
\item For the SE kernel, we have $a=0$ and hence in this case, we get the trivial bound $n_1 \leq n$. 
   
   
\item For \matern~kernels, we have $a = \frac{\tilde{D}}{\tilde{D} + 2\nu}$ where $\tilde{D} = D(D+1)$. We then have  three cases depending on the relative values of the smoothness parameter $\nu$ and the dimension $D$. 
\begin{itemize}
    \item If $2\nu < D(D+1)$, then $n_1 = \tOh{1}$. 
    \item If $D(D+1) \leq 2\nu < (D+1)(D+4)$, then $n_1 = o\lp n \rp$, i.e., $\lim_{n \to \infty} \frac{n_1}{n} = 0$. For simplicity, we will assume that $n$ is large enough to ensure that $n_1 \leq n$ in these cases. 
    
    \item If $2\nu> (D+1)(D+4)$ then we get the trivial bound $n_1 = \mc{O}(n)$. 
\end{itemize}
\end{itemize}
\end{proof}
